# Supplementary material for: The Power of Question Translation Training in Multilingual Reasoning: Broadened Scope and Deepened Insights
Source: arXiv:2405.01345 source file (2024-11-06)
Supplement: Supplementary file 1 [file 08_appendix.tex]

\section{Illustration of Evaluating the Consistency Between Reasoning Paths}
\label{sec:appendix}
In Table 5, we illustrate how we evaluate the reasoning consistency among reasoning process.
Specifically, we extract the last numerical value in each sentence as intermediate computation results and compute the Jaccard similarity between them as the consistency score of the reasoning paths.
